# Supplementary material for: Pre-training Tasks for User Intent Detection and Embedding Retrieval in E-commerce Search
Source: arXiv:2208.06150 source file (2022-08-22)
Supplement: Supplementary file 1 [file 7-appendix.tex]

\section{Appendix}

\begin{table}[htb]
\centering
\caption{Main results in P@K and N@K(small dataset).}
\label{table3}
\small
\setlength{\tabcolsep}{1mm}
\resizebox{.95\columnwidth}{!}{
\begin{tabular}{c|ccc|cc|ccc|cc}
\hline
\multirow{2}{*}{Method} & \multicolumn{5}{c|}{Overall} & \multicolumn{5}{c}{Long-tail} \\
\cline{2-11}
 & P@1 & P@3 & P@5 & N@3 & N@5 & P@1 & P@3 & P@5 & N@3 & N@5 \\
\hline
No pretrain (4-layer) & 0.862 & 0.408 & 0.265 & 0.870 & 0.884 & 0.764 & 0.305 & 0.191 & 0.837 & 0.851 \\
No pretrain (12-layer) & 0.861 & 0.405 & 0.265 & 0.867 & 0.882 & 0.757 & 0.305 & 0.190 & 0.834 & 0.847 \\
BERT-zh (12-layer) & 0.923 & 0.432 & 0.277 & 0.924 & 0.932 & 0.795 & 0.309 & 0.192 & 0.855 & 0.868 \\
Ours (4-layer) & 0.926 & 0.436 & 0.280 & 0.926 & 0.935 & 0.815 & 0.315 & 0.195 & 0.874 & 0.885 \\
Ours (12-layer) & $\mathbf{0.949}$ & $\mathbf{0.446}$ & $\mathbf{0.286}$ & $\mathbf{0.948}$ & $\mathbf{0.955}$ & $\mathbf{0.823}$ & $\mathbf{0.318}$ & $\mathbf{0.196}$ & $\mathbf{0.882}$ & $\mathbf{0.891}$ \\
\hline
\end{tabular}}
\vspace{-2mm}
\end{table}
